# Supplementary material for: A characterization of wreath products where knapsack is decidable
Source: arXiv:2101.06132 source file (2021-01-15)
Supplement: Supplementary file 1 [file appendix-h3-old.tex]

%

\section{Proof of \cref{lem:arithmetic}}

	We use vertical bars to indicate head power and underlining to define other loop conditions.
	The constraint $x = a$ is defined by $A^x A^{-a}$.
	The constraint $x = y$ is defined by $A^x \underline{A^{-*} \mid A^y} A^{-*}$.
	For addition we define
	\begin{equation}
		\label{eq:plus}
		C^x (BC)^* \underline{C^{-*} \underline{B^{-*} \mid B^y} C^{*}} B^{-*}
		\underline{C^{-*} \mid C^z} C^{-*}
	\end{equation}
	where stars stand for fresh variables.
	If $\nu$ satisfies $\nu(x) + \nu(y) = \nu(z)$ then $\nu$ can be extended to a solution of $\eqref{eq:plus}$
	since
	\[
		C^{\nu(x)} (BC)^{\nu(y)} \underline{C^{-\nu(z)} \underline{B^{-\nu(y)} \mid B^{\nu(y)}} C^{\nu(z)}} B^{-\nu(y)}
		\underline{C^{-\nu(z)} \mid C^{\nu(z)}} C^{-\nu(z)}
	\]
	is satisfied.
	Conversely, take a solution $\nu$ of \eqref{eq:plus}.
	Then by the knapsack equations and the interval constraints we obtain
	$C^{\nu(x)} (BC)^k C^{-\nu(z)} B^{-\nu(y)} = 1$ for some $k \in \Z$.
	Then we obtain $k = \nu(y)$ and therefore $\nu(x) + \nu(y) = \nu(z)$.
	
	For multiplication we use the fact that
	$A^u B^v A^{-w} B^{-x} = C^y$ if and only if $u=w$, $v=x$, and $y=uv$
	since the projections $H_3(\Z) \to \Z$ to the top-middle and the middle-right component
	are homomorphisms.
	We define:
	\begin{equation}
		\label{eq:times}
		A^x B^* A^{-*} \underline{B^{-*} C^{-*} \mid B^y C^*} \, \underline{C^{-*} B^{-*} \mid C^z B^*} B^{-*} C^{-*}
	\end{equation}
	Take an assignment $\nu$ with $\nu(x)\nu(y) = \nu(z)$.
	Then $\nu$ can be extended to a solution of $\eqref{eq:times}$ since
	\[
		A^{\nu(x)} B^{\nu(y)} A^{-{\nu(x)}} \underline{B^{-{\nu(y)}} C^{-{\nu(z)}} \mid B^{\nu(y)} C^{\nu(z)}} \, \underline{C^{-{\nu(z)}} B^{-{\nu(y)}} \mid C^{\nu(z)} B^{\nu(y)}} B^{-{\nu(y)}} C^{-{\nu(z)}}
	\]
	is satisfied.
	Conversely, take a solution $\nu$ of $\eqref{eq:times}$.
	Then by the knapsack equations and the interval constraints we obtain
	$A^{\nu(x)} B^{k} A^{-\ell} B^{-{\nu(y)}} C^{-{\nu(z)}} = 1$
	for some numbers $k,\ell \in \Z$.
	Therefore $\nu(x) = \ell$, $\nu(y) = k$ and $\nu(x)\nu(y) = \nu(z)$.

\section{Proof of \cref{lem:sync}}

	Let $\mathcal{V}' = \{x' \mid x \in \mathcal{V}\}$
	and let $S' = \{\nu' \in \Z^{\mathcal{V}'} \mid \nu'(x') = \nu(x) \text{ for all } x \in \mathcal{V} \}$.
	Suppose that $(E,I)$ and $(F,J)$ define the relations $R$ and $S'$.
	We juxtapose $E$ and $F$, combine the loop conditions
	from $I$ and $J$ (shifted by $|E|$) and the loop condition $(0,|E|)$.
	This new instance shows that intersection of $R$ and $S'$
	(viewed as relations in $\Z^{\mathcal{V} \cup \mathcal{V}'}$)
	is head definable.
	Hence, it remains to prove that, if $R$ is a head definable relation
	then also $\{\nu \in R \mid \nu(x_i) = \nu(x_j) \}$ is head definable for all $x_i,y_j \in R$.
	
	Suppose that $R$ is the set of integer solutions of $I = (E,L)$ restricted to $\mathcal{V}$.
	Assume that $E = e_1 \dots e_n$
	and that $e_i = g_i^{x_i}$ and $e_j = g_j^{x_j}$ are head powers in $I$.
	We first construct a new integer knapsack instance $I'$
	which contains head powers $g^x$ and $h^y$
	and expresses $x=y$.
	If $g \notin \langle C \rangle$ and $h \in \langle C \rangle$, or vice versa,
	then $g,h$ generate a free abelian group of rank 2
	and we can add to $\mathcal{E}$ the constraints
	\[
		g^x (g^{-1}h)^* \underline{h^{-*} \mid h^y} h^{-*}.
	\]
	Here every occurrence of $*$ represents a fresh variable.
	Otherwise we can find a matrix $M \in H_3(\Z) \setminus \{ 1 \}$
	such that $\langle g,M \rangle$ and $\langle h,M \rangle$
	are free abelian groups of rank 2.
	If $g,h \in \langle C \rangle$ we can choose $M = A$;
	if $g,h \notin \langle C \rangle$ we can choose $M = C$.
	Then we add to $\mathcal{E}$ the constraints
	\[
		g^x (g^{-1}M)^* \underline{M^{-*} \mid M^*} (hM^{-1})^* \underline{h^{-*} \mid h^y} h^{-*}.
	\]
	We can append $I'$ to $I$, and add the loop condition $(0,n)$
	and two loop conditions starting after $g_i^{x_i}$ ($g_j^{x_j}$)
	and ending on $g^x$ ($h^y$),
	which state that $x = x'$ and $y = y'$. This concludes the proof.
